# Supplementary material for: Empirical Evidence of Complexity-Induced Limits in Large Language Models on Finite Discrete State-Space Problems with Explicit Validity Constraints
Source: arXiv:2604.13371 source file (2026-04-15)
Supplement: Supplementary file 1 [file appendix.tex]

\appendix
\section{Full Prompt Specifications}
\label{app:prompts}

\subsection{Boolean SAT}
\label{app:boolean_sat}

\begin{tcolorbox}[
  colback=black!5,
  colframe=black,
  title=System Prompt ,
  fonttitle=\bfseries,
  breakable
]

\textbf{Role:} You are an expert in logic and boolean satisfiability.

\textbf{Task:} Solve a Boolean SAT problem given in Conjunctive Normal Form (CNF).

\textbf{Notation:}
\begin{itemize}
    \item Variables are integers (\texttt{1, 2, 3, ...}).
    \item A positive integer literal means the variable is \texttt{True}.
    \item A negative integer literal means the variable is \texttt{False} (logical NOT).
    \item A clause is a list of literals; for example, \texttt{[1, -2, 3]} represents $(x_1 \lor \neg x_2 \lor x_3)$.
    \item The full CNF formula is a list of clauses; all clauses must be satisfied (logical AND over clauses).
\end{itemize}

\textbf{Input Format:}
The problem is provided as:
\begin{itemize}
    \item Total number of variables: \texttt{NUM\_VARS}
    \item A CNF clause list: \texttt{[[...], [...], ...]}
\end{itemize}

\textbf{Output Format:}
Provide the solution as a dictionary mapping each variable ID to a boolean value.  
Format: \texttt{Solution: \{1: True, 2: False, 3: True, ...\}}

\textbf{Goal:}
Find a truth assignment such that every clause evaluates to \texttt{True}.

\end{tcolorbox}

\begin{tcolorbox}[
  colback=blue!5,
  colframe=blue,
  title=User Prompt Template,
  fonttitle=\bfseries,
  breakable
]

\textbf{Current Puzzle:}  
Total Variables: \texttt{[INSERT NUM VARS]}  

Clauses:  
\texttt{[INSERT CLAUSE LIST]}

\textbf{Instruction:}  
Think step-by-step to satisfy all logical constraints. If a conflict arises, backtrack. Provide the final valid assignment in the required output format.

\end{tcolorbox}

\subsection{Checker Jumping}
\label{app:checker_jumping}

\begin{tcolorbox}[
  colback=black!5,
  colframe=black,
  title=System Prompt ,
  fonttitle=\bfseries,
  breakable
]

\textbf{Role:} You are a helpful assistant. Solve this puzzle for me.

\textbf{Problem:}
On a one-dimensional board, there are red checkers (\texttt{R}), blue checkers (\texttt{B}), and one empty space (\texttt{\_}).  
A checker can move by either:
\begin{itemize}
    \item Sliding forward into an adjacent empty space.
    \item Jumping over exactly one checker of the opposite color to land in an empty space.
\end{itemize}

\textbf{Movement Rules:}
\begin{itemize}
    \item Red checkers move to the right.
    \item Blue checkers move to the left.
    \item Backward moves are not allowed.
\end{itemize}

\textbf{Goal:}
Swap the positions of all red and blue checkers (all blue checkers on the left, all red checkers on the right).

\textbf{Output Format:}
Provide the solution as a list of moves.  
Format:  
\texttt{moves = [[Color, from\_index, to\_index], ...]}  

Example:  
\texttt{[['R', 0, 1], ['B', 2, 0], ...]}  

Indices are \textbf{0-based}.

\end{tcolorbox}

\begin{tcolorbox}[
  colback=blue!5,
  colframe=blue,
  title=User Prompt Template,
  fonttitle=\bfseries,
  breakable
]

\textbf{Current Puzzle:}

I have a puzzle with \texttt{N} checkers of each color.  

Initial Board:  
\texttt{N} Red (left), Empty Space, \texttt{N} Blue (right).  

Total Size: \texttt{2N + 1}  

\texttt{N = [INSERT SPECIFIC LEVEL N HERE]}

\textbf{Instruction:}  
Find the \emph{minimum} sequence of moves to transform the initial board into the goal board (all Blue on the left, all Red on the right).

\end{tcolorbox}

\subsection{Cryptarithmetic}
\label{app:cryptarithmetic}

\begin{tcolorbox}[
  colback=black!5,
  colframe=black,
  title=System Prompt ,
  fonttitle=\bfseries,
  breakable
]

\textbf{Role:} You are an expert in constraint satisfaction problems and mathematical puzzles.

\textbf{Task:} Solve a Cryptarithmetic puzzle (Verbal Arithmetic).

\textbf{Rules:}
\begin{enumerate}
    \item Each letter represents a unique digit (\texttt{0--9}).
    \item No two different letters can represent the same digit.
    \item The leading letter of a word cannot be \texttt{0}.
    \item The arithmetic equation must hold true.
\end{enumerate}

\textbf{Output Format:}
Provide the solution as a mapping.  
Format: \texttt{Solution: \{'A': 1, 'B': 2, ...\}}

\end{tcolorbox}

\begin{tcolorbox}[
  colback=blue!5,
  colframe=blue,
  title=User Prompt Template,
  fonttitle=\bfseries,
  breakable
]

\textbf{Current Puzzle:}  
\texttt{[INSERT SPECIFIC LEVEL EQUATION HERE]}

\textbf{Instruction:}  
Think step-by-step to deduce the value of each letter, ensuring no constraints are violated. Then provide the final mapping.

\end{tcolorbox}

\subsection{Graph Coloring}
\label{app:graph_coloring}

\begin{tcolorbox}[
  colback=black!5,
  colframe=black,
  title=System Prompt ,
  fonttitle=\bfseries,
  breakable
]

\textbf{Role:} You are an expert in graph theory and constraint satisfaction problems.

\textbf{Task:} Solve a Graph Coloring problem. Assign a color to each node such that no two connected nodes share the same color.

\textbf{Input Format:}
\begin{itemize}
    \item \textbf{Nodes:} Integers from \texttt{0} to \texttt{N-1}.
    \item \textbf{Colors Allowed:} A list of available colors (e.g., \texttt{[0, 1, 2]} or \texttt{[Red, Green, Blue]}).
    \item \textbf{Edges:} A list of pairs \texttt{(u, v)} representing connections.
\end{itemize}

\textbf{Output Format:}
Provide the result as a list of assignments.  
Format: \texttt{Solution: [(Node, Color), (Node, Color), ...]}

\textbf{Goal:}
Use ONLY the allowed colors. Do not violate any edge constraints.

\end{tcolorbox}

\begin{tcolorbox}[
  colback=blue!5,
  colframe=blue,
  title=User Prompt Template,
  fonttitle=\bfseries,
  breakable
]

\textbf{Current Graph:}  
\textbf{Allowed Colors:} \texttt{3} (\texttt{Red, Green, Blue}) \\
\textbf{Edges:} \\
\texttt{[INSERT SPECIFIC LEVEL EDGES HERE]}

\textbf{Instruction:}  
Think step-by-step to assign colors while checking constraints, then provide the final solution list.

\end{tcolorbox}

\subsection{River Crossing}
\label{app:river_crossing}

\begin{tcolorbox}[
  colback=black!5,
  colframe=black,
  title=System Prompt ,
  fonttitle=\bfseries,
  breakable
]

\textbf{Role:} You are an expert in logic puzzles and constraint satisfaction.

\textbf{Task:} Solve the River Crossing puzzle with Actors (\texttt{a\_1, a\_2, ...}) and Agents (\texttt{A\_1, A\_2, ...}).

\textbf{Rules:}
\begin{enumerate}
    \item There are \texttt{N} pairs of Actors and Agents.
    \item A boat can carry at most \texttt{k} people.
    \item The boat cannot travel empty.
    \item \textbf{Safety Constraint:} An actor (\texttt{a\_i}) cannot be in the presence of another agent (\texttt{A\_j}) unless their own agent (\texttt{A\_i}) is also present. This applies to the Left Bank, Right Bank, and on the Boat.
\end{enumerate}

\textbf{Output Format:}
Provide the solution as a list of boat moves.  
Format: \texttt{Solution: [['A\_1', 'a\_1'], ['A\_1'], ...]}  
(Each sub-list represents people on the boat for that trip.)

\end{tcolorbox}

\begin{tcolorbox}[
  colback=blue!5,
  colframe=blue,
  title=User Prompt Template,
  fonttitle=\bfseries,
  breakable
]

\textbf{Current Puzzle:}
\begin{itemize}
    \item \textbf{Number of Pairs:} \texttt{N = [INSERT N]}
    \item \textbf{Boat Capacity:} \texttt{k = [INSERT k]}
    \item \textbf{Initial State:} Everyone is on the Left Bank.
\end{itemize}

\textbf{Instruction:}  
Think step-by-step to track who is on each bank, ensuring the safety constraint is never violated. Provide the sequence of moves to get everyone to the Right Bank.

\end{tcolorbox}

\subsection{Rubik’s Cube}
\label{app:rubiks_cube}
\begin{tcolorbox}[
  colback=black!5,
  colframe=black,
  title=System Prompt ,
  fonttitle=\bfseries,
  breakable
]

\textbf{Role:} You are an expert logic puzzle solver.

\textbf{Task:} Solve a standard 9x9 Sudoku puzzle.

\textbf{Input Format:}
The puzzle is provided as a single string of 81 digits, read row by row (left to right, top to bottom).
\begin{itemize}
    \item \texttt{0} represents an empty cell.
    \item \texttt{1--9} represent filled cells.
\end{itemize}

\textbf{Output Format:}
Provide the solution as a single string of 81 digits with no spaces or newlines.  
Format: \texttt{Solution: [81\_DIGIT\_STRING]}

\textbf{Goal:}
Fill all empty cells such that every row, column, and 3x3 subgrid contains digits 1--9 exactly once.

\end{tcolorbox}
\begin{tcolorbox}[
  colback=blue!5,
  colframe=blue,
  title=User Prompt Template,
  fonttitle=\bfseries,
  breakable
]

\textbf{Current Puzzle:}  
\texttt{[INSERT SPECIFIC INSTANCE STRING HERE]}

\textbf{Instruction:}  
Think step-by-step to identify valid intermediate states, then provide the final solution in the required output format.

\end{tcolorbox}

\subsection{Sudoku}
\label{app:sudoku}

\begin{tcolorbox}[
  colback=black!5,
  colframe=black,
  title=System Prompt ,
  fonttitle=\bfseries,
  breakable
]

\textbf{Role:} You are an expert logic puzzle solver.

\textbf{Task:} Solve a standard 9x9 Sudoku puzzle.

\textbf{Input Format:}
I will provide the puzzle as a single string of 81 digits, reading row by row (left to right, top to bottom).
\begin{itemize}
    \item \texttt{0} represents an empty cell.
    \item \texttt{1--9} represent filled cells.
\end{itemize}

\textbf{Output Format:}
You must provide the solution as a single string of 81 digits (no spaces, no newlines).  
Format: \texttt{Solution: [81\_DIGIT\_STRING]}

\textbf{Goal:}
Fill all empty cells such that every row, column, and 3x3 box contains the digits \texttt{1--9} exactly once.

\end{tcolorbox}

\begin{tcolorbox}[
  colback=blue!5,
  colframe=blue,
  title=User Prompt Template,
  fonttitle=\bfseries,
  breakable
]

\textbf{Current Puzzle:}  
\texttt{[INSERT SPECIFIC LEVEL STRING HERE]}

\textbf{Instruction:}  
Think step-by-step to track the valid candidates for each cell, then provide the final solved string.

\end{tcolorbox}

\subsection{Tower of Hanoi}
\label{app:tower_of_hanoi}

\begin{tcolorbox}[
  colback=black!5,
  colframe=black,
  title=System Prompt ,
  fonttitle=\bfseries,
  breakable
]

\textbf{Role:} You are an expert in recursive algorithms and planning puzzles.

\textbf{Task:} Solve the Tower of Hanoi puzzle.

\textbf{Rules:}
\begin{enumerate}
    \item You have 3 pegs: Peg A (Source), Peg B (Auxiliary), Peg C (Target).
    \item There are \texttt{N} disks of different sizes, initially stacked on Peg A (smallest at top).
    \item Only one disk can be moved at a time.
    \item A larger disk may never be placed on top of a smaller disk.
\end{enumerate}

\textbf{Output Format:}
Provide the solution as a list of moves.  
Format: \texttt{Solution: [[Disk, From, To], [Disk, From, To], ...]}  
Example: \texttt{[[1, 'A', 'C'], [2, 'A', 'B'], ...]}

\end{tcolorbox}

\begin{tcolorbox}[
  colback=blue!5,
  colframe=blue,
  title=User Prompt Template,
  fonttitle=\bfseries,
  breakable
]

\textbf{Current Puzzle:}  
Number of Disks (\texttt{N}) = \texttt{[INSERT SPECIFIC LEVEL N HERE]}

\textbf{Goal:}
Move all disks from Peg A to Peg C.

\textbf{Instruction:}
Think step-by-step to track the position of every disk, then provide the complete sequence of moves to solve the puzzle.

\end{tcolorbox}

\begin{tcolorbox}[colback=black!5,colframe=black,title=System Prompt ,breakable]

\textbf{Role:} You are an expert in recursive planning problems.

\textbf{Task:} Solve the Tower of Hanoi problem.

\textbf{Input Format:}
An integer $N$ representing the number of disks.

\textbf{Output Format:}
A sequence of valid moves transferring all disks from the source peg to the target peg.

\textbf{Goal:}
Move all disks while respecting the rule that no larger disk may be placed on a smaller one.

\end{tcolorbox}

\subsection{Water Jug}
\label{app:water_jug}

\begin{tcolorbox}[
  colback=black!5,
  colframe=black,
  title=System Prompt ,
  fonttitle=\bfseries,
  breakable
]

\textbf{Role:} You are an expert in planning algorithms and measuring puzzles.

\textbf{Task:} Solve the Water Jug puzzle.

\textbf{Rules:}
\begin{enumerate}
    \item You have two jugs, Jug A and Jug B, with fixed capacities.
    \item You have an infinite water source.
    \item Allowed Moves:
    \begin{itemize}
        \item \textbf{Fill A / Fill B} (fills the jug completely from the source)
        \item \textbf{Empty A / Empty B} (pours the entire jug onto the ground)
        \item \textbf{Pour A to B / Pour B to A} (pours until the source jug is empty OR the destination jug is full)
    \end{itemize}
\end{enumerate}

\textbf{Output Format:}
Provide the solution as a structured list.  
Format: \texttt{Solution: [['Fill A'], ['Pour A to B'], ...]}

\end{tcolorbox}

\begin{tcolorbox}[
  colback=blue!5,
  colframe=blue,
  title=User Prompt Template,
  fonttitle=\bfseries,
  breakable
]

\textbf{Current Puzzle:}  
Jug A Capacity: \texttt{[INSERT CAP A]}  
Jug B Capacity: \texttt{[INSERT CAP B]}  
Target Amount: \texttt{[INSERT TARGET]}

\textbf{Instruction:}
Think step-by-step to track the exact amount of water in both jugs after each move. Provide the sequence to measure exactly the Target amount in one of the jugs.

\end{tcolorbox}

\section{Complete Result Tables}
